# Supplementary material for: Precise Extraction of Deep Learning Models via Side-Channel Attacks on Edge/Endpoint Devices
Source: arXiv:2403.02870 source file (2024-03-05)
Supplement: Supplementary file 1 [file model_arch_vgg.tex]

\resizebox{0.7\columnwidth}{!}{
\begin{tabular}{c||c|c|c|c}
\toprule

{Model} & 
{\vggthree}&
{\vggsix}& 
{\vggonetwo} &
{\vggtwotwo}\\ 

\midrule
\hline

\multirow{1}{*}{conv1x}&
\multicolumn{4}{c}{
$\begin{bmatrix}
  \text{3x3, 64} \\
 \end{bmatrix}$
$\times 2$
}\\
\hline

\multirow{2}{*}{maxpool}&
\multirow{2}{*}{\xmark}&
\multirow{2}{*}{\xmark}& 
2x2&
2x2\\
&
&
&
stride 1& 
stride 2\\
\hline

\multirow{1}{*}{conv2x}&
\multicolumn{4}{c}{
$\begin{bmatrix}
  \text{3x3, 128} \\
 \end{bmatrix}$
$\times 2$
}\\
\hline

\multirow{2}{*}{maxpool}&
\multirow{2}{*}{\xmark}&
2x2&
2x2&
2x2\\
&
&
stride 2&
stride 2& 
stride 2\\
\hline

\multirow{1}{*}{conv3x}&
$\begin{bmatrix}
  \text{3x3, 128} \\
 \end{bmatrix}$
$\times 3$
&
\multicolumn{3}{c}{
$\begin{bmatrix}
  \text{3x3, 256} \\
 \end{bmatrix}$
$\times 3$
}\\
\hline

\multirow{2}{*}{maxpool}&
2x2&
2x2&
2x2&
2x2\\
&
stride 1&
stride 2&
stride 2& 
stride 2\\
\hline

\multirow{1}{*}{conv4x}&
$\begin{bmatrix}
  \text{3x3, 256} \\
 \end{bmatrix}$
$\times 3$
&
\multicolumn{3}{c}{
$\begin{bmatrix}
  \text{3x3, 512} \\
 \end{bmatrix}$
$\times 3$
}\\
\hline

\multirow{2}{*}{maxpool}&
2x2&
2x2&
2x2&
2x2\\
&
stride 2&
stride 1&
stride 2& 
stride 2\\
\hline

\multirow{1}{*}{conv5x}&
\multicolumn{4}{c}{
$\begin{bmatrix}
  \text{3x3, 512} \\
 \end{bmatrix}$
$\times 3$
}\\
\hline

\multirow{2}{*}{maxpool}&
\multicolumn{4}{c}{
2x2}\\
&
\multicolumn{4}{c}{
stride 2}\\
\hline

&
\multicolumn{4}{c}{
maxpool, FC, FC, FC, Softmax
}\\

\bottomrule 

\end{tabular}
}
