# Supplementary material for: Precise Extraction of Deep Learning Models via Side-Channel Attacks on Edge/Endpoint Devices
Source: arXiv:2403.02870 source file (2024-03-05)
Supplement: Supplementary file 2 [file model_hyperparams.tex]

\resizebox{\columnwidth}{!}{
\begin{tabular}{c||c|c|c|c|c|c}
\toprule

\revisionf{Analysis} & 
Type&
Model& 
Dataset &
LR &
WD&
Epoch
\\ 
\hline
\hline

\multirow{2}{*}{MA}&
Victim&
\multirow{2}{*}{$WRN28$-$k_{[32]}$}&
CIFAR-100&
\multirow{2}{*}{0.1}&
\multirow{2}{*}{5.00E-04.}&
200 \\
\cline{2-2}
\cline{4-4}
\cline{7-7}

&
Surrogate&
&
ImageNet&
&
&
100 \\
\hline

\multirow{10}{*}{ID}&
\multirow{8}{*}{Victim}&
\multirow{3}{*}{\resthree}&
Indoor67&
\multirow{2}{*}{0.05}&
\multirow{6}{*}{5.00E-04}&
\multirow{6}{*}{200} \\
\cline{4-4}

&
&
&
Caltech256&
&
&

\\
\cline{4-5}

&
&
&
CUB-200&
0.01&
&

\\
\cline{3-5}

&
&
\ressix&
\multirow{3}{*}{All}&
\multirow{3}{*}{0.1}&
&
\\
\cline{3-3}

&
&
\resonetwo
&
&
&
&
\\
\cline{3-3}

&
&
\restwotwo
&
&
&
&
\\
%%%resnet end 
\cline{3-7}

&
&
All VGG16&
\multirow{2}{*}{ImageNet}&
\multirow{2}{*}{0.001}&
\multirow{2}{*}{0.0005}&
\multirow{2}{*}{200}
\\

&
&
based models&
&
&
\\

\cline{2-7}

&
\multirow{4}{*}{Surrogate}&
All ResNet-50&
ImageNet&
\multirow{2}{*}{0.01}&
\multirow{2}{*}{0}&
\multirow{2}{*}{200}
\\
\cline{4-4}
&
&
based models&
OpenImages
&
&
&
\\
\cline{3-7}

%%%%%  vgg
&
&
All VGG16&
\multirow{2}{*}{ImageNet}&
\multirow{2}{*}{0.001}&
\multirow{2}{*}{0.0005}&
\multirow{2}{*}{200}
\\

&
&
based models&
&
&
\\

\bottomrule
\end{tabular}
}
